# Supplementary material for: Latent Bayesian Optimization via Autoregressive Normalizing Flows
Source: arXiv:2504.14889 source file (2025-04-21)
Supplement: Supplementary file 1 [file Generative_model_performance.tex]

\begin{table}[ht]
\centering
\caption{Performance Generative Model  Pretrained on Guacamol 1.27M Data.}
\label{table:generative_performance}
\begin{tabular}{c|c|c}
\midrule
Model & SeqFlow (Ours) (param=31,274,900)	 & TextFlow (param=54,760,765) \\
\hline
\midrule
Validity &	0.936 &	\textbf{0.975} \\
Uniqueness &	0.951 &	\textbf{0.995} \\
Novelty &	0.998 &	\textbf{0.999} \\
\midrule
\end{tabular}
\end{table}
